# Supplementary material for: gaBERT -- an Irish Language Model
Source: arXiv:2107.12930 source file (2022-06-28)
Supplement: Supplementary file 1 [file more-future-work.tex]

% appendix: more future work ideas

The following list of future work ideas has been collected from our
GitHub repository. \NOTE{Issue numbers refer to this repository.}
\begin{itemize}
    \item Effect of switching to v8 of Paracrawl \NOTE{issue \#77}
    \item Effect of random initialisation (using the same model type and settings as in the development phase; purpose is to find out whether the observed differences between settings are meaningful; differences that can be explained with model instability and that contradict expectations can then be disregarded)
    \item For each corpus, effect of removing it
    \item For each pair of corpora, effect of removing them
    \item Start with the NCI and add corpora in order of cleanliness (or data value estimate from above corpus ablation)
    \item More on filter thresholds and/or corpus-specific filter settings \NOTE{issue \#72}
    \item Effect of filtering (near) duplicates \NOTE{issue \#73}
    \item Effect of increasing the weight of clean corpora \NOTE{issue \#53}
    \item Restrict vocabulary building to clean corpora \NOTE{issue \#54}
    \item Partition the corpus, create a vocabulary for each partition and join the vocabularies \NOTE{issue \#33}
    \item Effect of \#\# glue on prefixes \NOTE{issue \#80}
    \item Effect of adding our in-house Irish Twitter corpora, in particular on tasks involving social media content \NOTE{issue \#34}
    \item Add a copy of the data with accents removed and/or other normalisations \NOTE{issue \#30}
    \item Add synthetic Irish, \eg MT output \NOTE{issue \#14}
    \item Add Hiberno-English corpora and English side of parallel corpora to training data \NOTE{issue \#13}
    \item The role of sentence-splitting, \eg does BERT need to see properly formed sentences or are snippets of text sufficient?
\end{itemize}
