# Supplementary material for: gaBERT -- an Irish Language Model
Source: arXiv:2107.12930 source file (2022-06-28)
Supplement: Supplementary file 2 [file reproducibility-checklist.tex]

\NOTE{We probably will have to complete the following checklist. Let's keep this here as a reminder.}
%
For all reported experimental results:
\begin{itemize}
    \item A clear description of the mathematical setting, algorithm, and/or model
    \item A link to a downloadable source code, with specification of all dependencies, including external libraries (recommended for camera ready, though welcome for initial submission)
    \TODO{Is this for the final version?
    Shouldn't this go into a supplement zip file in the submission?}
    \item A description of computing infrastructure used
    \item The average runtime for each model or algorithm, or estimated energy cost
    \item The number of parameters in each model
    \item Corresponding validation performance for each reported test result    
    \item A clear definition of the specific evaluation measure or statistics used to report results. 
\end{itemize}

\noindent
For all results involving multiple experiments, such as hyperparameter search:
\begin{itemize}
    \item The exact number of training and evaluation runs
    \item The bounds for each hyperparameter
    \item The hyperparameter configurations for best-performing models
    \item The method of choosing hyperparameter values (e.g. manual tuning, uniform sampling, etc.) and the criterion used to select among them (e.g. accuracy)
    \item Summary statistics of the results (e.g. mean, variance, error bars, etc.)
\end{itemize}
    
\noindent
For all datasets used:
\begin{itemize}
    \item Relevant statistics such as number of examples and label distributions
    \item Details of train/validation/test splits
    \item An explanation of any data that were excluded, and all pre-processing steps
    \item For natural language data, the name of the language(s)
    \item A link to a downloadable version of the dataset or simulation environment
    \TODO{Venues that strictly require all used data sets to be publicly available will not
    be suitable for our NCI-based work. What top conferences still are open to us?} 
\end{itemize}
